# Supplementary material for: InstantEdit: Text-Guided Few-Step Image Editing with Piecewise Rectified Flow
Source: arXiv:2508.06033 source file (2025-08-08)
Supplement: Supplementary file 1 [file supp_diverse_edit.tex]

\begin{figure*}[h]
 \centering
 \begin{minipage}{\textwidth}
\includegraphics[width=\linewidth]{figs/supp_diverse_edit.pdf}
\caption{ Additional editing results with diverse text prompts.
\label{fig:supp_diver_edit}
}
\end{minipage}
\end{figure*}
